# Supplementary material for: Few-shot NeRF by Adaptive Rendering Loss Regularization
Source: arXiv:2410.17839 source file (2024-10-23)
Supplement: Supplementary file 1 [file supp_T_k.tex]

\begin{tabular}{l|c|c|c|c|c}
\toprule
  & &  PSNR $\uparrow$ & SSIM $\uparrow$ & LPIPS $\downarrow$ & Average $\downarrow$  \\
  \midrule
\multirow{3}{*}{$T_s$} 
& 8000 & 20.21 & 0.773 & 0.214 & 0.103 \\
& 10000 & 20.07 & 0.773 & 0.215 & 0.103 \\
& 12000 & 20.09 & 0.774 & 0.214 & 0.105 \\
\midrule\midrule
\multirow{3}{*}{$k$} & 3 & 20.07 & 0.773 & 0.215 & 0.103 \\
& 5 & 19.84 & 0.772 & 0.214 & 0.105 \\
& 7 & 19.38 & 0.764 & 0.220 & 0.113 \\
\bottomrule
\end{tabular}
