# Supplementary material for: Few-shot NeRF by Adaptive Rendering Loss Regularization
Source: arXiv:2410.17839 source file (2024-10-23)
Supplement: Supplementary file 2 [file supp_dtu.tex]

\begin{tabular}{l|c|c|c|c|c}
\toprule
Method & Year & {PSNR $\uparrow$} & {SSIM $\uparrow$} & {LPIPS $\downarrow$} & {Average $\downarrow$} \\
\midrule
DietNeRF~\cite{jain2021putting} & ICCV2021 & 11.85 & 0.633 & 0.314 & 0.243 \\
RegNeRF~\cite{niemeyer2022regnerf} & CVPR2022 & 18.89 & 0.745 & 0.190 & 0.112 \\
MixNeRF~\cite{seo2023mixnerf} & CVPR2023 & 18.95 & 0.744 & 0.228 & 0.118 \\
FreeNeRF~\cite{yang2023freenerf} & CVPR2023 & \cellcolor{orange!25}19.92 & \cellcolor{orange!25}0.787 & \cellcolor{red!25}0.182 & \cellcolor{orange!25}0.098 \\
FlipNeRF~\cite{seo2023flipnerf} & ICCV2023 & \cellcolor{yellow!25}19.55 & 0.767 & 0.206 & \cellcolor{yellow!25}0.107 \\
SparseNeRF~\cite{wang2023sparsenerf} & ICCV2023 & \cellcolor{yellow!25}19.55 & \cellcolor{yellow!25}0.769 & \cellcolor{yellow!25}0.201 & - \\
\textbf{AR-NeRF (Ours)} & - & \cellcolor{red!25}20.36 & \cellcolor{red!25}0.788 & \cellcolor{orange!25}0.187 & \cellcolor{red!25}0.095 \\
\bottomrule
\end{tabular}
