# Supplementary material for: Few-shot NeRF by Adaptive Rendering Loss Regularization
Source: arXiv:2410.17839 source file (2024-10-23)
Supplement: Supplementary file 3 [file supp_llff.tex]

\begin{tabular}{l|c|c|c|c|c}
\toprule
Method & Year & {PSNR $\uparrow$} & {SSIM $\uparrow$} & {LPIPS $\downarrow$} & {Average $\downarrow$} \\
\midrule
DietNeRF~\cite{jain2021putting} & ICCV2021 & 14.94 & 0.370 & 0.496 & 0.240 \\
RegNeRF~\cite{niemeyer2022regnerf} & CVPR2022 & 19.08 & 0.587 & 0.336 & 0.146 \\
MixNeRF~\cite{seo2023mixnerf} & CVPR2023 & 19.27 & 0.629 & \cellcolor{orange!25}0.301 & \cellcolor{yellow!25}0.135 \\
FreeNeRF~\cite{yang2023freenerf} & CVPR2023 & \cellcolor{yellow!25}19.63 & 0.612 & \cellcolor{yellow!25}0.308 & \cellcolor{orange!25}0.134 \\
FlipNeRF~\cite{seo2023flipnerf} & ICCV2023 & 19.34 & \cellcolor{orange!25}0.631 & 0.312 & 0.136 \\
SparseNeRF~\cite{wang2023sparsenerf} & ICCV2023 & \cellcolor{orange!25}19.86 & \cellcolor{yellow!25}0.624 & 0.328 & - \\
\textbf{AR-NeRF (Ours)} & - & \cellcolor{red!25}19.90 & \cellcolor{red!25}0.635 & \cellcolor{red!25}0.283 & \cellcolor{red!25}0.126 \\
\bottomrule
\end{tabular}
