# Supplementary material for: Few-shot NeRF by Adaptive Rendering Loss Regularization
Source: arXiv:2410.17839 source file (2024-10-23)
Supplement: Supplementary file 4 [file supp_model_size_inference_time.tex]

\begin{tabular}{l|c|c|c}
\toprule
  & PSNR $\uparrow$ & Model size (MB) $\downarrow$ & Inference time (s) $\downarrow$ \\
  \midrule
Mip-NeRF & 8.69 & 7.4 & 5.434 \\
% RegNeRF & 18.89 & 0.770($1.62\times10^{-5}$) & 0.217($5.56\times10^{-6}$) \\
MixNeRF & 18.95 & 7.4 & 5.402 \\
FreeNeRF & 19.92 & 7.4 & 5.448 \\
\textbf{Ours (AR-NeRF)} & {\bf 20.36} & 7.4 & 5.424 \\
\bottomrule
\end{tabular}
