# Supplementary material for: Few-shot NeRF by Adaptive Rendering Loss Regularization
Source: arXiv:2410.17839 source file (2024-10-23)
Supplement: Supplementary file 5 [file supp_universality.tex]

\begin{tabular}{l|c|c|c}
\toprule
  &  PSNR $\uparrow$ & SSIM $\uparrow$ & LPIPS $\downarrow$ \\
  \midrule
SparseNeRF & 18.96 & 0.624 & 0.328 \\
SparseNeRF+FreeNeRF & 20.26 & 0.646 & 0.292 \\
\textbf{SparseNeRF+Ours (AR-NeRF)} & \bf 20.45 & \bf 0.670 & \bf 0.271 \\
\bottomrule
\end{tabular}
